# Supplementary material for: Hybrid photovoltaic and electron-tunneling converters
Source: arXiv:1409.3300 source file (2014-09-11)
Supplement: Supplementary file 1 [file Supplementary.pdf]

# Supplementary information for hybrid photovoltaic and electron-tunneling converters

Shanhe Su<sup>1</sup>, Jincan Chen<sup>1</sup>, Tien-Mo Shih<sup>2</sup>

<sup>1</sup>Fujian Key Laboratory of Semiconductor Materials and Applications and Department of Physics, Xiamen University, Xiamen 361005, People's Republic of China

<sup>2</sup>Institute for Complex Adaptive Matter, University of California, Davis, CA 95616, USA

In this supplementary, computations of the equilibrium Fermi level and the electron concentration are described. The photoexcited electron concentration is computed and used to obtain the cathode current density on the basis of the balance equation. The energy conservation equation over both the cathode and the absorber will be established to govern the cathode temperature.

## Fermi level and electron concentration in equilibrium

For a p-type semiconductor cathode, such as boron-doped silicon at a given  $E_g$  and  $T_C$ , the equilibrium Fermi level  $E_f$  and the electron concentration  $n_{eq}$  without illumination can be numerically computed by the charge neutrality in the semiconductor crystal<sup>1</sup>

$$n_{eq} + N_A^- = p_{eq}, \quad (S1)$$

where  $n_{eq} = N_C e^{-(E_c - E_f)/k_B T_C}$  is the electron concentration;  $N_A^- = N_A \frac{1}{1 + 4e^{(E_A - E_f)/k_B T_C}}$

the ionised concentration for the boron acceptor using Boltzmann statistics as an approximation;  $p_{eq} = N_V e^{-(E_f - E_v)/k_B T_C}$  the hole carrier concentration;  $E_c$  the energy at

the conduction-band minimum;  $E_v$  the energy at the valence-band maximum;  $E_A = 0.044 \text{ eV}$  the ionisation energy of the boron acceptor in silicon at acceptor impurities of concentration  $N_A = 10^{19} \text{ cm}^{-3}$  [Refs. 1, 2];  $N_C = 2 \left( 2\pi m^* k_B T_C / h^2 \right)^{3/2}$  the effective densities of states in the conduction band;  $N_V = 2 \left( 2\pi m_p^* k_B T_C / h^2 \right)^{3/2}$  the effective densities of states in valence band;  $m^* = 1.0 m_e$  the effective mass of electrons;  $m_p^* = 0.57 m_e$  the effective mass of hole carriers; and  $m_e$  the mass of an free electron. In setting  $E_v = 0$ , Eq. (S1) can be rewritten as

$$N_C e^{-(E_g - E_f)/k_B T_C} + N_A \frac{1}{1 + 4e^{(E_A - E_f)/k_B T_C}} = N_V e^{-E_f/k_B T_C}. \quad (\text{S2})$$

### Photoexcited electron concentration and cathode current density

Based on  $J = e / 2\pi \int_0^\infty N(\mu, T) \zeta(E_x) dE_x$  and  $N(\mu, T) = [m^* k_B T / (\pi \hbar^3)] \exp[-(E_x - \mu) / (k_B T)]$ ,

the electrical current density  $J_C$  flowing from the cathode to the anode is given by

$$J_C = \frac{e}{2\pi} \frac{m^* k_B T_C}{\pi \hbar^3} \int_0^\infty \exp\left(-\frac{E_x - E_{f,n}}{k_B T_C}\right) \zeta(E_x) dE_x, \quad (\text{S3})$$

where the quasi-Fermi level is defined as  $E_{f,n} = E_f + k_B T_C \ln(n / n_{eq})$ . Substituting the expression of  $E_{f,n}$  into Eq. (S3) and rewriting the cathode current density in terms of the photoexcited electron concentration  $n$  lead to

$$J_C = \frac{e}{2\pi} \frac{m^* k_B T_C}{\pi \hbar^3} \frac{n}{n_{eq}} \int_0^\infty \exp\left(-\frac{E_x - E_f}{k_B T_C}\right) \zeta(E_x) dE_x = \Gamma_C n. \quad (\text{S4})$$

The rate of the photon-enhanced recombination per unit volume in Eq. (4) can be expressed as

$$R = \frac{1}{L} \frac{1}{n_{eq} p_{eq}} \frac{2\pi}{h^3 c^2} \int_{E_g}^\infty \frac{(h\nu)^2 d(h\nu)}{e^{h\nu/k_B T_C} - 1} (np - n_{eq} p_{eq}) = \Gamma_R (np - n_{eq} p_{eq}). \quad (\text{S5})$$

Upon inserting Eqs. (S4) and (S5) into Eq. (3), the relation that determines the photoexcited electron concentration  $n$  can be obtained as

$$G + \frac{J_A}{eL} = \Gamma_R(np - n_{eq}p_{eq}) + \frac{\Gamma_C n}{eL}. \quad (\text{S6})$$

Under illumination, values of conduction- and valence-band concentrations deviated from the equilibrium concentration counterpart are given by

$$\Delta n = \Delta p = n - n_{eq} = p - p_{eq}. \quad (\text{S7})$$

Equation (S6) can be rewritten as

$$\Gamma_R \Delta n^2 + \left[ \Gamma_R (n_{eq} + p_{eq}) + \frac{\Gamma_C}{eL} \right] \Delta n - \left( G + \frac{J_A}{eL} - \frac{\Gamma_C}{eL} n_{eq} \right) = 0, \quad (\text{S8})$$

where  $\Delta n$  can be directly obtained by solving Eq. (S8). Photoexcited electron concentration  $n = n_{eq} + \Delta n$  is then inserted into Eq. (S4) to determine the cathode current density  $J_C$ .

### Energy balance and temperatures of both the cathode and the absorber

The temperature  $T_C$  is governed by the energy conservation over the cathode and the absorber. A layer of solar-absorbing material coated on the top of the cathode allows sub-bandgap photons to be absorbed to become thermal energy, and is completely transparent to supra-bandgap photons. The absorbed solar energy  $P_{sun}$  either leaves the cathode through the tunnel or reemits by the radiative recombination. The net heat flux density  $Q_{net}$  exiting the cathode is computed by noting that an electron leaving the electrode removes thermal energy equal to the difference between its total energy and the electrochemical potential of the electrode<sup>3</sup>. A fraction of  $Q_{net}$  is available to be converted to electric power  $J_{net} \times V$ , while the remainder is lost due to the irreversibility. The energy balance of the cathode is given by

$$P_{sun} = Q_{net} + P_{rad} + P_{n,rad} + P_{sa}. \quad (S9)$$

Each electron traveling from the cathode to the anode carries the energy of  $E_x + k_B T_C - E_F$ , where  $k_B T_C$  is the average value of free energy in the transverse plane based on the Maxwell-Boltzmann statistics. Likewise, an electron carries the energy of  $E_x + k_B T_A - E_F$  in the reverse direction<sup>4</sup>. Therefore, by combining with Eq.

(2), the net heat flux density carried by electrons through the tunnel is

$$Q_{net} = \frac{1}{2\pi\hbar} \int_0^\infty \left[ (E_x + k_B T_C - E_F) N(E_{F,n}, T_C) - (E_x + k_B T_A - E_F) N(E_{F(A)}, T_A) \right] \zeta(E_x) dE_x. \quad (S10)$$

The emissivity of the cathode is assumed to be unity within the spectrum  $[E_g, \infty]$ . The equilibrium radiative recombination energy loss  $P_{rad}$  in the cathode<sup>5</sup> is given by

$$P_{rad} = \frac{2\pi}{h^3 c^2} \int_{E_g}^\infty \frac{(h\nu)^3 d(h\nu)}{e^{h\nu/k_B T_C} - 1}. \quad (S11)$$

Because photoexcited populations of electrons and holes are larger than their equilibrium counterpart, the cathode radiative recombination under illumination is larger than that in equilibrium. The photon-enhanced radiative recombination energy flux is expressed by

$$P_{n,rad} = \left( \frac{np}{n_{eq} p_{eq}} - 1 \right) \frac{2\pi}{h^3 c^2} \int_{E_g}^\infty \frac{(h\nu)^3 d(h\nu)}{e^{h\nu/k_B T_C} - 1}, \quad (S12)$$

and the radiation  $P_{sa}$  emitted from solar-absorbing material is given by

$$P_{sa} = \frac{2\pi}{h^3 c^2} \int_0^{E_g} \frac{(h\nu)^3 d(h\nu)}{e^{h\nu/k_B T_C} - 1}. \quad (S13)$$

## References

1. Sze, S.M. *Physics of semiconductor devices 2nd edn* (Wiley, 1981).
2. Schwede, J.W. et al. Photon-enhanced thermionic emission for solar concentrator systems. *Nature Mater.* **9**, 762 – 767 (2010).
3. Humphrey, T.E., Newbury, R., Taylor, R.P. & Linke, H. Reversible quantum Brownian heat engines for electrons. *Phys. Rev. Lett.* **89**, 116801 (2002).
4. O'Dwyer, M.F., Lewis, R.A., Zhang, C. & Humphrey, T.E. Electronic efficiency in nanostructured thermionic and thermoelectric devices. *Phys. Rev. B* **72**, 205330 (2005).
5. Würfel, P. *Physics of solar cells: From basic principles to advanced concepts 2nd edn* (Wiley-VCH, 2009).
